# Supplementary material for: Entanglement between a telecom photon and an on-demand multimode solid-state quantum memory
Source: arXiv:2106.05079 ancillary file (2021-11-23)
Supplement: Supplementary file 1 [file Supplementary_Material.pdf]

# Supplemental Material: Entanglement between a telecom photon and an on-demand multimode solid-state quantum memory


Jelena V. Rakonjac,[1,*] Dario Lago-Rivera,[1,*] Alessandro Seri,[1]
Margherita Mazzera,[2] Samuele Grandi,[1,†] and Hugues de Riedmatten[1,3]

[1] *ICFO-Institut de Ciencies Fotoniques, The Barcelona Institute of Science and Technology, 08860 Castelldefels (Barcelona), Spain*

[2] *Institute of photonics and quantum sciences, SUPA, Heriot-Watt University, Edinburgh, EH14 4AS, UK*

[3] *ICREA-Institució Catalana de Recerca i Estudis Avançats, 08015 Barcelona, Spain*



(Dated: November 23, 2021)


This Supplemental Material contains additional information regarding the experiment:

**Section I:** detailed information about the entanglement source and the quantum memory, and comparison with our previous work.

**Section II:** characterisation of the entanglement analyzers, and discussion on the advantages and disadvantages of the different solid-state interferometers.

**Section III:** limitations to the measurable values of visibilities.

**Section IV:** analysis of AFC and spin-wave storage efficiencies, and signal-to-noise level.

**Section V:** description of the model for visibility verus storage time in the spin state.

## I. SETUP

The setup, as shown in Fig. S1, consists of two main parts: the photon-pair source and the quantum memory. These will be described in subsec. I A and I B, respectively.

### A. Source

The source of entangled photon pairs is based on cavity-enhanced spontaneous parametric down-conversion (cSPDC), as previously described in [1–3]. The pump laser at 426 nm (generated through frequency doubling from an 852 nm seed laser - TOPTICA TA-SHG 110) is sent to a cavity containing a periodically-poled lithium niobate crystal (PPLN), generating a photon with a wavelength of 1436 nm (the idler) and another at 606 nm (the signal). A homebuilt Fabry-Perot reference cavity (Locking Cavity) is used to lock the seed laser to reduce the laser linewidth such that the coherence time of the laser is much longer than the coherence time of the biphoton ($\tau_{\mathrm{pump}} \gg \tau_{\mathrm{biphoton}}$). To ensure that the signal photon is resonant with the Pr transition used for the memory, the length of the cavity is locked to a 606 nm reference beam (resonant with the AFC) with a piezo-electric actuated mirror (PZ). The idler photon is kept resonant to the cavity by using feedback from a classical beam at 1436 nm generated in the same PPLN crystal through difference frequency generation (DFG) between the pump beam and the reference 606 nm beam. The feedback acts to tune the pump laser wavelength by adjusting the position of one of the reference cavity mirrors with a piezo-actuator to change the cavity length, and since the seed is locked to the cavity, the wavelength will follow the change. A mechanical chopper at the output of the SPDC cavity is used to alternate between locking the setup and measuring single photons to avoid sending classical light to the SPDs. The cycle has a period of 33 ms, with a measurement duty cycle of 55%. The resulting pump laser linewidth is 380(20) kHz, corresponding to $\tau_{\mathrm{pump}} \approx 1\mu$s, determined using the idler interferometer in Section II A, and the biphoton linewidth is 1.8 MHz.

After the output of the source cavity, the signal and idler paths are separated with a dichroic mirror. As the spectrum of the photons is composed of several frequency modes [2], the idler photon is first sent to a filter cavity (FCav) to ensure single-mode operation. Filtering of broadband noise is provided by a bandpass filter (BPF, central wavelength 1440 nm, linewidth 14 nm). The signal photon also passes through a bandpass filter (central wavelength 600 nm, linewidth 10 nm) for broadband filtering before being sent to the memory.

The idler photon is then sent to the fiber-based idler interferometer. Details regarding the interferometer can be found in Section II A. Finally, the photon is sent to a superconducting nanowire single photon detector (ID281, ID Quantique), which has a detection efficiency of 80% and 14 Hz of dark counts. Under current experimental conditions, spurious light increases the background rate to 120 Hz.

---


* These two authors contributed equally.
† samuele.grandi@icfo.eu

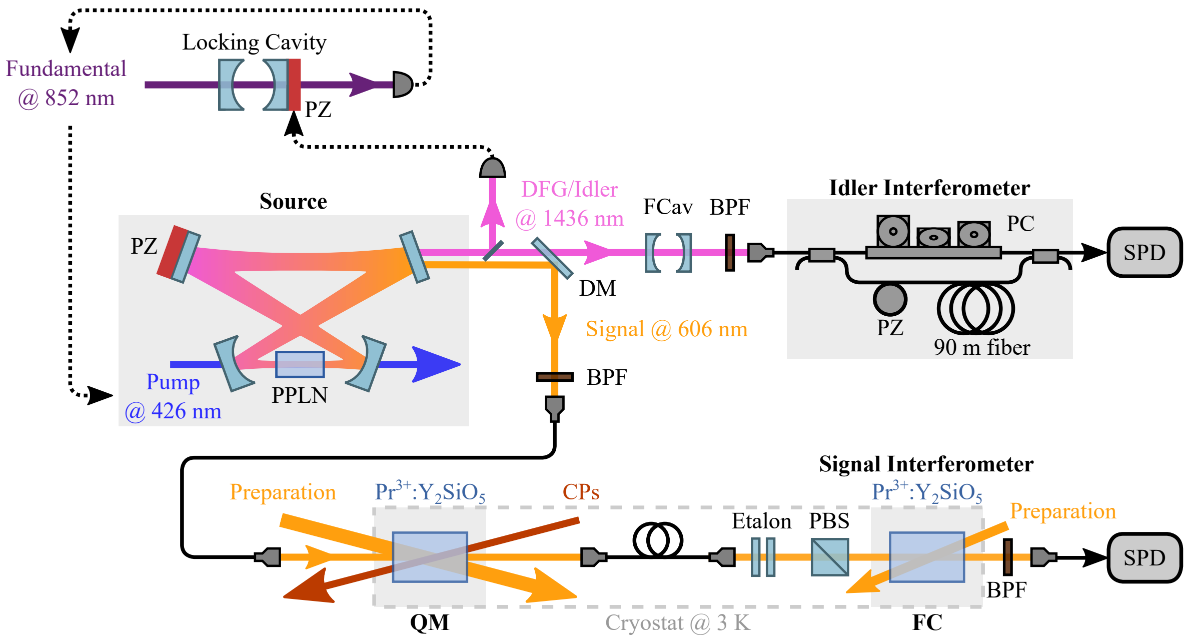


FIG. S1. Experimental setup showing the photon pair source, the locking system for the pump laser, the quantum memory (QM) setup and the two interferometers. The individual components used are: piezoelectric actuators (PZ), periodically-poled lithium niobate (PPLN), dichroic mirror (DM), filter cavity (FCav), bandpass filter (BPF), polarization controller (PC), polarizing beamsplitter (PBS), the $Pr^{3+}$:$Y_2SiO_5$ filter crystral (FC) and single photon detectors (SPD). CPs (control pulses) indicate the control pulse beam path.

### B. Memory

For the memory setup, we use two $Pr^{3+}$:$Y_2SiO_5$ crystals (grown by Scientific Materials): one as the quantum memory (QM) and another as the filter crystal (FC), which doubles as an unbalanced Mach-Zehnder interferometer (UZMI) for the signal photons. Both crystals are doped with 0.05% $Pr^{3+}$ ions and have dimensions of $2 \times 3 \times 5$ mm, corresponding to the $D_1$, $D_2$ and $b$ refractive index axes, respectively. All light is propagated along the $b$ axes of the crystals, and polarized along the $D_2$ axis. Both crystals are cooled to 2.7 K in the same closed-cycle cryostat (Optistat AC-V14, Oxford Instruments). The cryostat imparts strong vibrations on the cold finger and thus any crystals attached to it. These vibrations cause strain induced shifts and broadening of the ions in the crystal which limit the quality of the AFC structure we can prepare. Thus, we place the two crystals on a homebuilt sample mount with springs to decouple the crystal from the vibrations, allowing us to achieve longer storage times with higher efficiencies [3].

We only address Pr ions in the crystallographic site 1 in these experiments. We use a frequency doubled laser from 1212 nm to 606 nm (Toptica TA-SHG) to address the ions in the crystal. The laser is locked to a homebuilt Fabry-Perot reference cavity at 1212 nm using the Pound-Drever-Hall technique, with an estimated linewidth of no more than 10 kHz. All the preparation light for the memory crystal and the filter crystal is generated with double-pass acousto-optics modulators (AOMs), controlled by a fast Arbitrary Waveform Generator (Signadyne/Keysight).

The signal photons are focused inside the QM to a waist of 40 $\mu$m. Two separate paths are used to prepare the AFC structure and apply the control pulses (CPs), with beam waists of approximately 180 $\mu$m and 100 $\mu$m, respectively. The CP path is intentionally counterpropagating and at an angle to the signal photon path to reduce noise at the single photon detector. The signal photon is then sent to the FC via a single-mode optical fiber, again with a waist of 40 $\mu$m inside the crystal. A separate beam path (waist 200 $\mu$m) is used to prepare a transparency window, or an AFC if the FC is used as the signal interferometer.

Spectral filtering of the CPs is performed using three main components, as described in the main text: the FC, the BPF, and the etalon. The FC has an inhomogeneous linewidth of 10 GHz [1], and is used to filter the light from the CP field which is 10.2 MHz away from the signal photons, as well as fluorescence from the $3/2_e$ level to the $3/2_g$ and $5/2_g$ levels (fluorescence to the $1/2_g$ level cannot be filtered). The BPF is used to filter broadband light at other wavelengths, including fluorescence induced from the CPs from the $^1D_2(0)$ level to other crystal field levels in the $^3H_4$ manifold. The solid fused silica etalon (free spectral range 100 GHz, finesse 23.5) can filter light in the region between the cutoff of the inhomogenenous line of the FC and the BPF, which is again likely to come from fluorescence decay to other crystal field levels in $^3H_4$, and broadband noise from the source. Addition-

ally, a PBS (which is also part of the polarization control of the signal path) filters unpolarized fluorescence noise from the CPs. Finally, the photons are detected with a single photon counter (COUNT-10C-FC for AFC measurements and COUNT-50C-FC for SW measurements, Laser Components). The timestamps of detection events, from both signal and idler photons, are recorded using a Time-to-Digital Converter (Signadyne).

Note that for the AFC interference fringes shown in the main text, and the interference fringe without the QM in Section II C, the etalon was placed before the input fiber to the QM, and the signal photon traveled from the QM to the FC in free space through two single-pass AOMs instead of an optical fiber. For these two measurements, the $g^{(2)}_{s,i}$ through a transparency window in the QM was 24(1), and $g^{(2)}_{AFC,i}$ was 61(7). The decrease of $g^{(2)}_{AFC,i}$ with respect to the value quoted in the main text was due to the AFC not yet being well-optimized (thus being less efficient) at the time of the interference fringe measurements.

We prepare the AFC in a similar manner to that described in Ref. [4] for a 10 $\mu$s storage time. First, we prepare a 20 MHz wide spectral pit, then bring back population to this region by applying a burn-back pulse on the $5/2_g$ to $5/2_e$ transition. We apply a cleaning pulse close to the $3/2_g$ to $3/2_e$ transition in order to obtain a single class absorption feature corresponding to the $1/2_g$ to $3/2_e$ transition. To prepare the AFC structure, we use a parallel preparation method similar to Ref. [5], but we instead simulate our desired comb structure, take its Fourier transform and apply this temporal waveform to the spectral feature. We apply this waveform at 4 points in frequency, 1 MHz apart, in order to prepare a uniform structure over the 4 MHz comb bandwidth. To ensure that the $3/2_g$ level is kept empty, we alternate between applying the temporal waveform to burn the AFC and applying cleaning pulses on the $3/2_g$ to $3/2_e$ transition. Finally, we apply stronger cleaning pulses on the $3/2_g$ to $3/2_e$ transition which have the same power, waveshape, frequency span and central frequency as the CPs for further cleaning. For the CPs and the final cleaning pulses, we use pulses with a Gaussian amplitude, which have a full width half maximum of 2.5 $\mu$s, and a hyperbolic tangent frequency chirp which spans 4.2 MHz. The preparation procedure takes a total of 366 ms. A trace of the AFC structure can be seen in Fig. S2, along with the spectral pit used for the FC. Finally, when performing semi-conditional spin-wave storage, we optimized the number $N$ of pairs of control pulses such as to obtain a statistically significant error on the $g^{(2)}$ in the shortest time. We found that the optimum is normally achieved for $N = g^{(2)}$. This means that the value of $N$ was different for every point of the interference fringes shown in Fig. 2(b) of the main text

As mentioned in the main text, the efficiency of AFC storage alone is 19.7(6)%, and 6.2(3)% with SW storage, as measured with single photons as the input. The coincidence rates in the window of the echo (at the signal detector) are 3.8 Hz and 0.062 Hz for AFC and SW storage, respectively. The SW coincidence rate is much lower than that of the AFC due to the detection dead time imposed by the semiconditional SW storage sequence (4.4 ms for every idler detected). If we instead consider the number of coincidences (at the signal detector) per idler detected, we measure $3.8 \cdot 10^{-3}$ and $1.2 \cdot 10^{-3}$ coincidences per idler for AFC and SW storage, respectively. The AFC echo coincidence rate is nearly 60 times higher than our previous work [4], in part due to using a detector for the idler that is 8 times more efficient, but otherwise due to improvements in the experiment, while the SW echo rate is only about 3 times higher, again due to the dead time imposed by the experiment. We have listed a comparison with our previous work [4] in Table I.

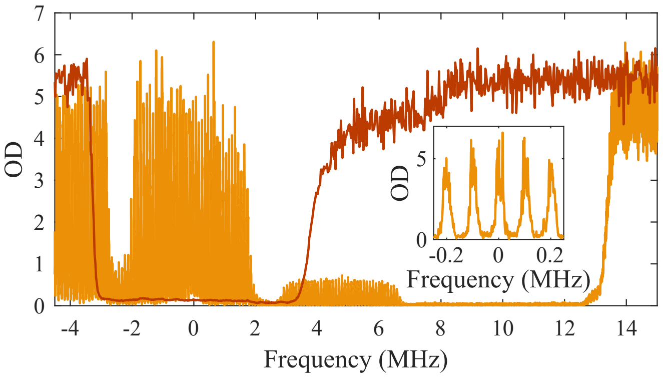


FIG. S2. The AFC structure (orange) prepared in the QM and the spectral pit used for filtering prepared in the FC (red). The frequency detuning is given relative to the input photon frequency. The inset shows a zoom-in of a small region of frequency of the AFC.

## II. ANALYZERS

### A. Idler interferometer

The fiber-based idler interferometer consists of a short arm with a polarization controller and a long arm with a home-made fiber stretcher (a cylindrical piezo-actuator with optical fiber wrapped around it) and an additional 90 m of optical fiber. The corresponding path length difference in time is 424 ns.

The phase of the idler interferometer is controlled by the fiber stretcher. Applying a voltage to the piezo-actuator stretches the fiber, thus changing its length and the phase difference between the short and long paths. To lock the interferometer to a specific phase, we scan the phase of the interferometer and observe a classical DFG signal at 1436 nm, then lock to a particular point with a side-fringe lock. We use a set point in the lower half of the fringe as it is less sensitive to power fluctuations. To shift to another interferometer phase, a con-

| | $\Delta\nu_{pump}$ | $\Delta\nu_{bi\text{-}ph}$ | $T_2^{eff}$ | $\eta_{AFC}$ ($\tau_{AFC}$) | $\eta_T$ | $\gamma_{inhom}$ | $T_S$ | Noise Floor | $g^{(2)}_{SW,i\ (320ns)}$ |
|---|---|---|---|---|---|---|---|---|---|
| Ref. [4] | > 1 MHz | 2.8 MHz | 33 $\mu$s | 11.0(5)% (7.5 $\mu$s) | 72.5% | 20(3) kHz | 6 $\mu$s | $1.3 \cdot 10^{-3}$ | 4.96 |
| This work | 380(20) kHz | 1.8 MHz | 92(9) $\mu$s | 19.7(6)% (10 $\mu$s) | 64.4% | 16.1(7) kHz | 6.9 $\mu$s | $0.83(4) \cdot 10^{-3}$ | 9.19 |

TABLE I. Comparison with our previous work [4]. $\Delta\nu_{pump}$: linewidth of source pump laser; $\Delta\nu_{bi\text{-}ph}$: linewidth of the idler-signal bi-photon; $T_2^{eff}$: effective coherence time of the AFC storage [5]; $\eta_{AFC}$ ($\tau_{AFC}$): efficiency of the AFC for storage time $\tau_{AFC}$; $\eta_T$: control pulse transfer efficiency; $\gamma_{inhom}$: spin state inhomogeneous broadening; $T_S$: storage time in the spin state; $g^{(2)}_{SW,i\ (320ns)}$: semi-conditional cross-correlation function.

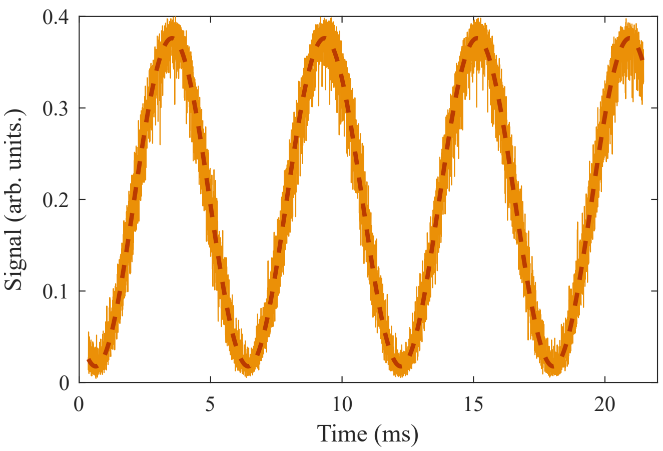


FIG. S3. Transmission through one output of the fiber-based idler interferometer over time while the phase is scanned continuously. The 1436 nm DFG light was used as the input. The dashed line corresponds to a sinusoidal fit used to obtain the visibility, with a value of 91.3(7) %.

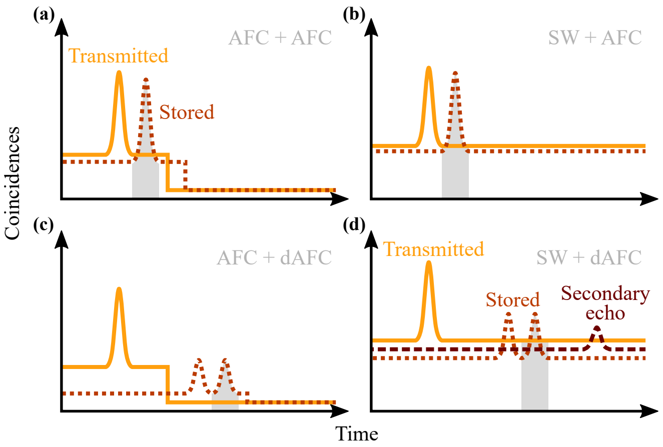


FIG. S4. Visual representation of the role of noise in different signal interferometers. The grey shaded area represents the region that will be used to measure interference. (a) and (c): single- and double-AFC interferometer for AFC storage. The double-AFC interferometer is preferred, as it moves the echoes away from the stored SPDC noise, that drops off right after the transmitted peak due to the pump laser being switched off. (b) and (d): single- and double-AFC interferometer for SW storage. Here a single-AFC interferometer is preferred, as the broad noise from the CPs is transmitted or stored (and re-emitted) with equal probability to the signal photons.

stant voltage is added to the applied signal during the measurement phase. The interferometer is locked during the same locking phase of the SPDC source.

To determine the visibility of the idler interferometer we use a well-stabilized 1535 nm laser as the input, and scan the interferometer. From the minimum and maximum values of the output, we estimate the visibility to be larger than 99%, limited by unequal losses between the long and short arms of the interferometer. We repeat this measurement using the 1436 nm classical DFG light and obtain a visibility of 91.3(7)% by fitting a sinusoid to the transmission of one output of the interferometer (see Fig. S3). The reduction in visibility is to be expected due to the larger linewidth of the 426 nm laser. This is because, as mentioned previously, the DFG light is generated using the 606 nm and 426 nm lasers, and thus its linewidth is dependent on both. Since the 606 nm light has a narrow linewidth, a measurement with the DFG light will be limited by the 426 nm laser. Using the measured value for the visibility, and a Gaussian model for the phase noise, we can estimate the laser linewidth of the 426 nm pump to be 380(20) kHz [6].

## B. Signal interferometer

As described in the main text, we use the FC in the setup as the interferometer for the signal photons. This interferometer is based on the output of either two superimposed AFCs referred to as a “double AFC” (for excited state storage; see Fig. S5) or a single AFC echo and the transmitted light (for SW storage; see Fig. S6). We use a different type of interferometer for these two cases due to differences in the background noise. A visual explanation of the reason is shown in Fig. S4.

For the double AFC interferometer and SW storage (see Fig. S4(d)), the signal we consider for our interference measurements will only be stored and emitted by the 2 $\mu$s and 2.42 $\mu$s AFCs, but the noise from the CPs can either be transmitted through the double AFC, stored and emitted for the two aforementioned storage times or at one of the secondary echoes, clearly visible in see Fig. S5(b). Moreover, the efficiencies of the 2 $\mu$s and 2.42 $\mu$s combs are 10% each, while for SW storage

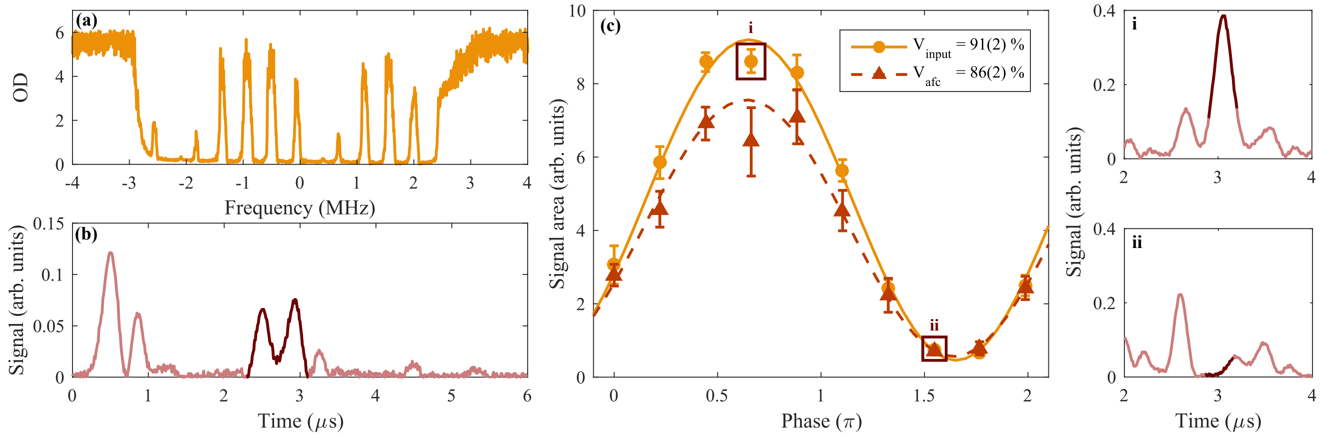


FIG. S5. (a) OD vs frequency for a double AFC structure, where zero frequency detuning corresponds approximately to the input photon frequency. (b) Temporal spectrum of the double AFC from (a) with a single classical pulse as the input. The darker region of the trace indicates the two echoes used as the short and long interferometer, while the other peaks come from the transmitted light (first peak) or other smaller echoes or secondary echoes. (c) Interference fringes measured using the double AFC interferometer for classical pulses either transmitted through a transparency window in the QM, or stored in an AFC in the QM. The insets i and ii correspond to a maximum and minimum of interference respectively through a transparency window in the QM, where the area used for the points of the fringe is darkened.

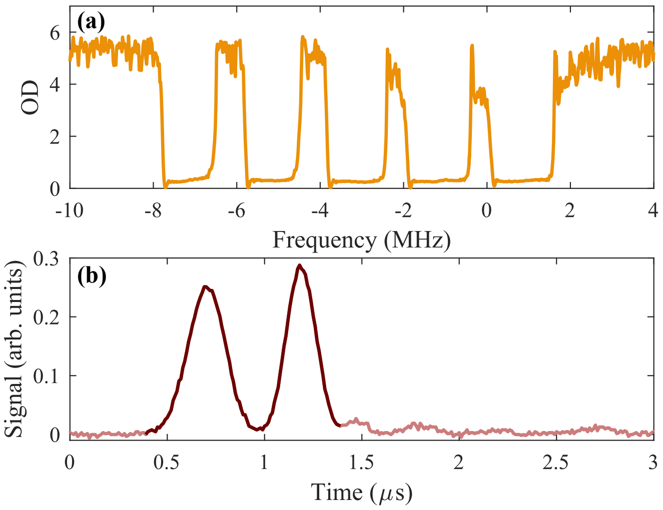


FIG. S6. (a) OD vs frequency for the single AFC structure, used as an interferometer when performing spin-wave storage. Zero frequency detuning corresponds approximately to the input photon frequency. (b) Temporal spectrum of the AFC from (a) with a single classical pulse as the input. The darker region of the trace indicates the peaks corresponding to the transmitted and stored light, used as the short and long interferometer paths respectively.

60% of the noise (mostly due to the control pulses) will pass through the FC, therefore reducing the maximum $g^{(2)}_{SW,i}$ and thus the visibility of the interference. Therefore, for SW storage we use the transmitted and stored photons of a single AFC as the short and long paths respectively. Unlike the double AFC interferometer, there are minimal secondary echoes, and so the signal photons are transmitted with a similar efficiency as the noise photons [see Fig. S4(b)]. The storage efficiency of the single AFC is optimized to be similar to that of the transmitted light through the comb, which is approximately 25% for both. This allows the $g^{(2)}_{SW,i}$ at the phase of maximum interference to be similar to that of $g^{(2)}_{SW,i}$ measured without interferometers. Despite the larger storage efficiency, the single AFC interferometer is not suitable for excited state storage as the interference window is in a temporal position where there is still stored noise from the pump laser, which will limit the visibility due to a reduction in $g^{(2)}_{AFC,i}$(see Fig. S4(a)). This is not a problem in the case of SW storage because the CP noise dominates all other sources of noise and so the stored pump noise in that temporal window is negligible. To compare, approximately 60% of the noise can be transmitted or stored by the double AFC (but 10% can be stored in one echo), whereas 50% of the noise can be transmitted or stored in the single AFC and 25% of the signal can be stored in one temporal path. It is therefore better to use a double AFC interferometer.

To prepare the AFC for either of the FC interferometers, we use a more simplified sequence compared to the QM as no class cleaning is required. In both cases, we first prepare a 6 MHz wide spectral pit centered at the QM AFC frequency. We then burn back population using the $5/2_g$ to $5/2_e$ transition. Then we prepare a comb using the serial holeburning method [5]. For the double AFC, we alternate repeatedly between burning a 2 $\mu$s and 2.4 $\mu$s comb. The preparation of this comb is optimized such that a photon can be stored for either time with equal probability. The final structure is then centered to the AFC of the QM. For the single AFC, we simply burn one comb. The storage time was chosen such that the echo is separated from the transmitted light by

as close to 424 ns as possible. In this case, the separation between the teeth, $\Delta$, is 2 MHz, corresponding to a 500 ns storage time and due to slow light effects, the delay between transmitted light and echo is close to 424 ns. Similarly to the double AFC, the storage efficiency is optimized such that light can be transmitted or stored with equal probability. This AFC is not centered with the QM AFC, but instead extends approximately 7.4 MHz lower in frequency and 2 MHz higher in frequency, to avoid approaching the fluorescence from transitions at higher frequencies than the input photons.

To scan the phase of these interferometers, we shift the position in frequency where the 2.4 $\mu$s comb is burnt for the double AFC, and similarly we shift the position of the comb for the single AFC interferometer. For each phase, we reoptimize the AFC sequence to equalize the probability of the photon traveling along either the short or long path, and maintain similar storage efficiencies across all the phases used.

Figure S5(b) shows interference fringes measured with classical pulses for storage with and without the memory. We use two classical light pulses, separated by 424 ns as the input, and measure the interference as a function of the change of the double AFC phase, $\Delta\phi_s$. For a transparency window in the QM crystal, the visibility is 91(2)%. For AFC storage, the visibility is 86(2)%. In comparison, we measured visibilities of 90(3)% and 88(3)% with single photons in the main text. We would expect the visibilities to be smaller when measured with single photons due to the pump laser linewidth. This discrepancy could be due to the input used to measure the classical fringes, which may not be equivalent in shape or temporal separation to the single photons.

One consequence of using the double AFC as an interferometer is that we do not have a temporal window of noise (equivalent to the noise where we measure interference) with which we can calculate $g^{(2)}_{s,i}$ or $g^{(2)}_{AFC,i}$. To calculate $g^{(2)}_{s,i}$ we typically use a temporal window before the transmitted signal photon where the pump is turned on. To calculate $g^{(2)}_{AFC,i}$, we consider a temporal window after the pump has been turned off but before the AFC echo has been emitted, where there is only stored pump noise. If only the double AFC is used for example, then we should consider a noise window after the pump is switched off but before the first echo, but due to the non-instantaneous switching off of the pump, there is no such window. This is also the case if there is also an AFC in the memory. Hence, we must use a noise window before the transmitted signal (if there is a spectral pit prepared in the memory) or before the AFC echo (if there is an AFC preparation in the memory) that would have more noise counts than the temporal window in which we measure interference. This would underestimate $g^{(2)}_{s,i}$ and $g^{(2)}_{AFC,i}$, so instead we refer to this value as the normalized coincidences in the main text. This is also why the normalized coincidences are below one at the minimum of the interference fringes in Fig S7 and Fig. 2 in the main text.

### C. Interference without QM storage

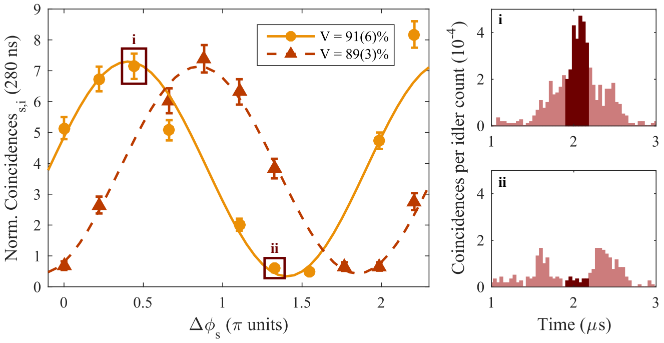


FIG. S7. Interference fringe measured with single photons with the signal passing through a transparency window in the QM. Each fringe is measured by fixing the idler interferometer phase and sweeping the signal interferometer phase for two idler interferometer phases differing in phase by $\pi/2$. The insets i and ii correspond to a maximum and minimum of interference, corresponding to the points indicated on the fringe, and the shaded regions indicate the counts used for the fringe.

We can verify the combined performance of our two analyzers by measuring energy-time entanglement of the photon pair alone, without storage in the QM. To do this, we prepare a 16 MHz wide spectral pit in the QM, and double-AFC in the FC for the signal interferometer. The resulting interference fringe is shown in Fig. S7. We measure visibilities of 91(6) % and 89(3) %, showing that the photons are entangled as expected.

## III. LIMITATIONS TO THE MEASURABLE VISIBILITY

For the spin-wave storage experiment, with perfect analyzers, for our measured $g^{(2)}_{SW,i}$ of 9.8(6), we should be able to measure an interference fringe with a visibility of 81%. However, our measured visibility is lower. From Section II A, we know the idler interferometer visibility (for 1436 nm light generated with the 426 nm pump laser) is 91(3)%. From a measurement using classical input and using the minimum and maximum values of interference only, we can also estimate the visibility of the single AFC interferometer to be 87.4%. This value accounts for imperfection in the visibility due to the trade-off between the width of the temporal modes and their separation: from a simulated set of data, this could amount to a maximum visibility of 95% to 91%. Overall, we would expect to measure a visibility of 65%, which is very close to our measured values. The difference between the expected and measured values could be due to an imperfect estimation of the single AFC interferometer visibility, for

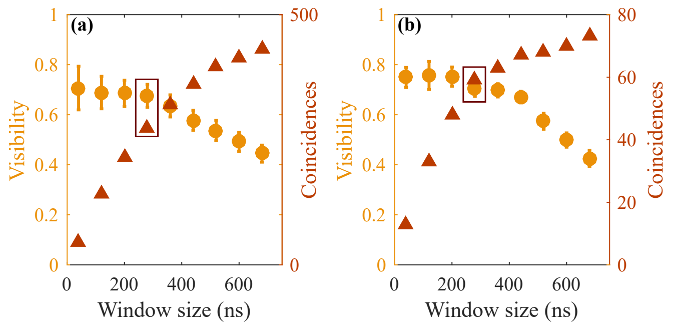


FIG. S8. Interference visibility and number of coincidences at the maximum of interference versus windows size for the interference fringes measured after SW storage. The boxes indicate the window size selected and shown in the main text, which correspond to the visibilities (a) 68(5) % and (b) 71(3) %.

example. In the case of the signal interferometer, a fiber-based interferometer should perform better, with a visibility close to 99% (as shown in Section II A). We chose to use a solid-state implementation as the setup is much simpler (no additional optical or electronic components are needed compared to a spin-wave storage experiment) and more stable as no locking is required. Even with a perfect signal analyzer, our expected visibility (due to the source pump laser and the current value of $g^{(2)}_{SW,i}$) would be 74%, which would make it difficult to exceed the 71% threshold for violating a CHSH inequality within experimental error. An improved linewidth or $g^{(2)}_{SW,i}$ would thus be required. A new laser or better locking cavity would be needed to improve the linewidth. Section IV will discuss the limiting factors of our AFC efficiency and $g^{(2)}_{SW,i}$.

The visibility is also affected by the temporal window we use to calculate $g^{(2)}_{SW,i}$. Figure S8 shows the visibility versus window size (for a fixed central time bin) for the two fringes measured, as well as the corresponding number of coincidences at the phase of maximum interference. We chose to use a window size of 280 ns as a good balance between visibility and count rate, since we can increase the visibility by using a smaller window at the expense of decreasing the count rate.

## IV. EFFICIENCY ANALYSIS

The expected efficiency for a particular AFC structure depends on the optical depth (OD), background absorption and finesse of the comb. Deviations from the ideal finesse due to imperfect comb preparation can lead to a reduced AFC efficiency. For Gaussian comb peaks, the expected internal efficiency is given by: [7]

$$\eta_{AFC} = \widetilde{d}^2 e^{-\frac{7}{F^2}} e^{-\widetilde{d}} e^{-d_0}, \tag{1}$$

where $\widetilde{d}$ is the effective optical depth given by $OD/F$, $F$ is the finesse of the comb, and $d_0$ is the absorption background which comes from imperfect optical pumping. For the comb we prepare, $OD = 4.1(3)$, $F = 3.4(1)$ and $d_0 = 0.18 \pm 0.11$. The expected efficiency from these values is 20(3)%.

The ideal comb peak shape is that of a square, rather than Gaussian. Then the expected efficiency is: [8]

$$\eta_{AFC} = \widetilde{d}^2 e^{-\widetilde{d}} \mathrm{sinc}^2\left(\frac{\pi}{F}\right) e^{-d_0}. \tag{2}$$

We can calculate the maximum possible efficiency for this storage time assuming that the optical pumping is perfect, i.e., maintain the same $OD$ and comb period $\Delta$, but reduce $d_0$ to zero and shape the comb teeth with square tops and a finesse that maximizes the efficiency. For our system, $F = 3.9$ maximizes the efficiency with a value of 33%. Due to bandwidth mismatch, 25% of the input photon will be lost, thus limiting the maximum storage efficiency (for 10 $\mu$s) measurable with our setup to about 25%. To further increase $\eta_{AFC}$, we could use a multipass setup of the input through the crystal, or an impedance-matched cavity [9].

The SW efficiency, which directly affects $g^{(2)}_{SW,i}$, is related to the AFC efficiency $\eta_{AFC}$ according to

$$\eta_{SW} = \eta_{AFC}\, \eta_T^2\, \eta_C \tag{3}$$

where $\eta_T$ is the transfer efficiency of a single control pulse, and $\eta_C$ denotes the proportion of the signal remaining after decoherence from the Gaussian inhomogeneous broadening of the hyperfine levels. The decay is given by $\eta_C = exp(-\frac{(T_s \gamma_{\mathrm{inhom}})^2}{2ln(2)}\pi^2)$, so for our storage time $T_s = 6.9$ $\mu$s, $\eta_C = 0.93$. In our case, the largest loss in $\eta_{SW}$ is from $\eta_T$. We can determine $\eta_T$ by sending a single control pulse and observing the decrease in the AFC echo efficiency:

$$\eta_T = 1 - \frac{\eta'_{AFC}}{\eta_{AFC}} \tag{4}$$

where $\eta'_{AFC}$ is the AFC efficiency after applying a single control pulse. For the control pulses used in our experiments, $\eta_T = 64.4(4)\%$. We can easily increase $\eta_T$ by using more power for our control pulses for example. However, this will result in the generation of more noise unless we have perfectly emptied the population of the $3/2_g$ level. Our control pulse power was chosen specifically to maximize the signal-to-noise ratio (SNR) for experiments using weak coherent pulses as an input, which should correspond to a maximum in $g^{(2)}_{SW,i}$. Figure S9 shows how both the noise floor and SW echo efficiency increase with respect to control pulse power, but in terms of $\mu_1$, defined as the ratio between the number of input photons per pulse and the signal to noise ratio, $\mu_1 = \frac{n_{input}}{SNR}$, the minimum occurs for a power of 8.5 mW, which is what we used for the experiments in this paper. Further optimization of the temporal and spectral shape of the CPs is required in order to obtain a higher $\eta_T$ without increasing the noise floor, which would then

result in a larger $g^{(2)}_{SW,i}$. Note that if we can improve the AFC efficiency, $g^{(2)}_{SW,i}$ will also improve even without any improvement in $\eta_T$.

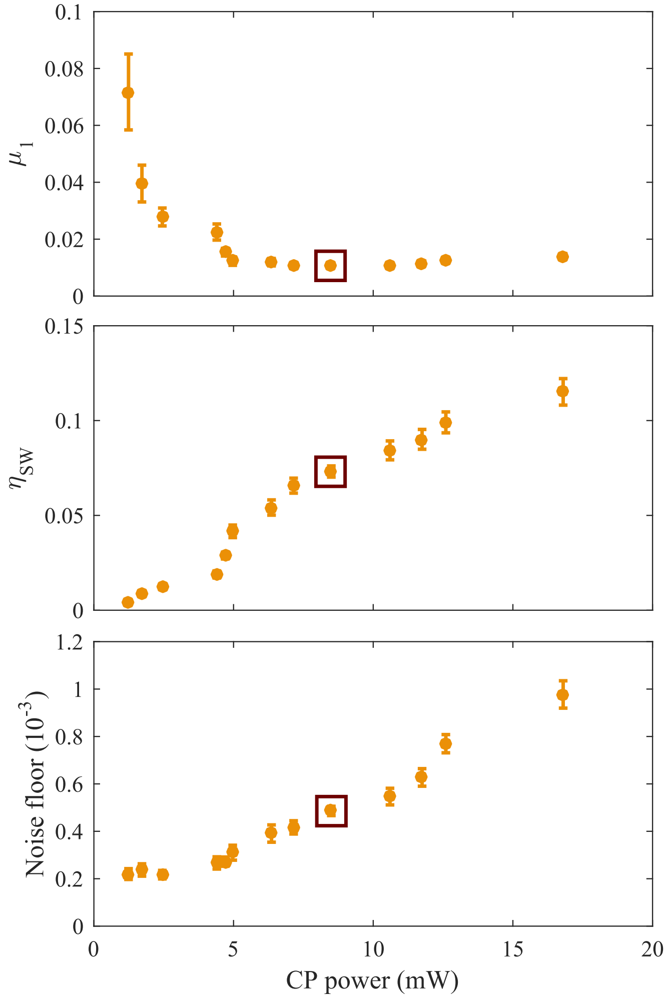


FIG. S9. Measurements of (a) $\mu_1$, (b) spin-wave storage efficiency $\eta_{SW}$ and (c) noise floor (in 500 ns) versus applied control pulse power using weak coherent pulses as an input. For these measurements, the number of input photons per pulse was approximately 0.36. The points corresponding to the power used for the measurements with single photons as an input are indicated with a box.

## V. MODELLING VISIBILITY VERSUS STORAGE TIME

We will now introduce the model that we use to explain the dependence of the entanglement visibility $V$ with the time that the signal photon spends in the spin-state $T_s$. The starting point is the ideal dependence of the visibility with the second order cross-correlation function $g^{(2)}_{s,i(\Delta t)}$:

$$V = \frac{g^{(2)}_{s,i(\Delta t)} - 1}{g^{(2)}_{s,i(\Delta t)} + 1}. \quad (5)$$

For SW storage, $g^{(2)}_{SW,i(\Delta t)}$ depends on $T_s$ according to the formula [10]

$$g^{(2)}_{SW,i(\Delta t)} = g^{(2)}_{s,i(\Delta t),0} \cdot \frac{SNR(T_s) + 1}{SNR(T_s) + g^{(2)}_{s,i(\Delta t),0}} \quad (6)$$

where $g^{(2)}_{s,i(\Delta t),0}$ corresponds to the second order cross-correlation after an AFC storage and $SNR(T_s) \propto \eta_{SW}(T_s)$ is the signal-to-noise of the signal mode after spin-wave retrieval. In our case, we can now assume that $SNR(T_s) \ll g^{(2)}_{s,i(\Delta t),0}$ and use the equation $\eta_{SW} = a_\eta \cdot e^{-\frac{(T_s \cdot \gamma_{inhom} \cdot \pi)^2}{2 \cdot \log(2)}}$ in order to get the final equation for the second order cross-correlation after SW storage of:

$$g^{(2)}_{SW,i(\Delta t)} = a_{g^{(2)}} \cdot e^{-\frac{(T_s \cdot \gamma_{inhom} \cdot \pi)^2}{2 \cdot \log(2)}} + 1. \quad (7)$$

Here, $\gamma_{inhom}$ represents the spin state inhomogeneous broadening which, after fitting to experimental data, corresponds to $\gamma_{inhom} = 14.8(9)$ kHz. In addition, note that $a_{g^{(2)}} = 10.2(9)$, meaning that $g^{(2)}_{SW,i(\Delta t)} = 11.2(9)$ for the case with $T_s = 0$. However, equation (5) assumes an experiment only limited by photon correlations. In reality several factors will lead into imperfect interference, like non-idealities in the analyzers or limited quality of the initial entangled state. This means that the minimum of interference will not correspond to 1 anymore as equation (5) assumes, but to a larger number. Usually, we could account for this by adding an extra parameter $\eta$

$$V = \eta \cdot \frac{g^{(2)}_{s,i(\Delta t)} - 1}{g^{(2)}_{s,i(\Delta t)} + 1}. \quad (8)$$

The problem in our case is that depending on $T_s$ not only the value of $g^{(2)}_{SW,i(\Delta t)}$ for the maximum of interference will change, but also the value of $g^{(2)}_{SW,i(\Delta t)}$ for the minimum will decrease over time. In this direction, we introduce a new parameter $b$. We do it in such a way that the value of $g^{(2)}_{SW,i(\Delta t)}$ in the minimum of interference for $T_s = 0$ will correspond to $b + 1$. The parameter $b$ represents the extra contribution to the minimum of interference due to imperfect experimental parameters (mode mismatch, pump coherence time etc). Additionally, we will make this value sensitive to the spin inhomogeneity using a similar formula to equation (7). Applying these modifications, we get

$$V = \frac{(a_{g^{(2)}} - b) \cdot e^{-\frac{(T_s \cdot \gamma_{inhom} \cdot \pi)^2}{2\log(2)}}}{(a_{g^{(2)}} + b) \cdot e^{-\frac{(T_s \cdot \gamma_{inhom} \cdot \pi)^2}{2\log(2)}} + 2} \quad (9)$$

For obtaining the fit that appears in Fig. 3(c) of the main text, we use the values of $a$ and $\gamma_{inhom}$ that we obtained in Fig. 3(b) of the main text, i.e., $b$ is the only free parameter of this fit with $b = 0.8(3)$.

As a final note, we would like to point out that while the value of $g^{(2)}_{SW,i}$ for the point at $T_S = 37.7$ $\mu$s is below 2, in fact it is 1.8(6), the non-classicality of the correlations between the idler and the retrived spin-wave is ensured by the visibility of 44(8)% that we measured, that is also compatible with the measured $g^{(2)}_{SW,i}$. Moreover, the classical limit is set by the Cauchy-Schwarz parameter $R = \left(g^{(2)}_{SW,i}\right)^2 / \left(g^{(2)}_{i,i} \cdot g^{(2)}_{SW,SW}\right)$, that is the ratio between the cross-correlation function between idler and retrieved spin-wave and the product between the cross-correlation functions of the idler and of the signal modes individually. In ref. [4] we measured $g^{(2)}_{i,i} = 1.32(4)$ and $g^{(2)}_{SW,SW} = 1.0(4)$. While we did not measure the auto-correlation functions, it is possible to obtain a value $R > 1$ even with a $g^{(2)}_{SW,i} < 2$ [1, 2, 4].


[1] A. Seri, G. Corrielli, D. Lago-Rivera, A. Lenhard, H. de Riedmatten, R. Osellame, and M. Mazzera, Laser-written integrated platform for quantum storage of heralded single photons, Optica **5**, 934 (2018).

[2] A. Seri, D. Lago-Rivera, A. Lenhard, G. Corrielli, R. Osellame, M. Mazzera, and H. de Riedmatten, Quantum Storage of Frequency-Multiplexed Heralded Single Photons, Physical Review Letters **123**, 080502 (2019).

[3] D. Lago-Rivera, S. Grandi, J. V. Rakonjac, A. Seri, and H. de Riedmatten, Telecom-heralded entanglement between multimode solid-state quantum memories, Nature **594**, 37 (2021).

[4] A. Seri, A. Lenhard, D. Rieländer, M. Gündoğan, P. M. Ledingham, M. Mazzera, and H. de Riedmatten, Quantum Correlations between Single Telecom Photons and a Multimode On-Demand Solid-State Quantum Memory, Physical Review X **7**, 021028 (2017).

[5] P. Jobez, N. Timoney, C. Laplane, J. Etesse, A. Ferrier, P. Goldner, N. Gisin, and M. Afzelius, Towards highly multimode optical quantum memory for quantum repeaters, Physical Review A **93**, 032327 (2016).

[6] J. Minar, H. de Riedmatten, C. Simon, H. Zbinden, and N. Gisin, Phase-noise measurements in long-fiber interferometers for quantum-repeater applications, Phys. Rev. A **77**, 052325 (2008).

[7] M. Afzelius, C. Simon, H. de Riedmatten, and N. Gisin, Multimode quantum memory based on atomic frequency combs, Physical Review A **79**, 052329 (2009).

[8] M. Bonarota, J. Ruggiero, J. L. L. Gouët, and T. Chanelière, Efficiency optimization for atomic frequency comb storage, Physical Review A **81**, 033803 (2010).

[9] M. Afzelius and C. Simon, Impedance-matched cavity quantum memory, Physical Review A **82**, 022310 (2010).

[10] B. Albrecht, P. Farrera, X. Fernandez-Gonzalvo, M. Cristiani, and H. de Riedmatten, A waveguide frequency converter connecting rubidium-based quantum memories to the telecom c-band, Nature Communications **5**, 3376 (2014).
